# Supplementary material for: Self-Binarizing Networks
Source: arXiv:1902.00730 source file (2019-02-02)
Supplement: Supplementary file 1 [file 70_Appendix.tex]

\section{Appendices}

\subsection{Appendix.A XNORNet Adaptations for $\tanh$}
\label{ap:XnornetGC}

\PMN{It feels like this appendix comes out of nowhere. Either we explain exactly how this is related to our work or we should remove it.}

\newcommand{\myW}{\mathrm{\textbf{W}}}
\newcommand{\myB}{\mathrm{\textbf{B}}}

In XNORNet, the $\sign$ function is scaled by $\alpha$ in the forward pass in order to minimize the difference between the floating point weights $\mathrm{\textbf{W}}$ and their binary representation $\mathrm{\textbf{B}}$:
\begin{equation}
\alpha = \underset{\alpha > 0, \myB}{\text{argmin}} ||\myW - \alpha \myB||
\end{equation}
The optimal $\alpha$ value would be:
\begin{equation}
\label{eq:alpha-tanh}
\alpha = \frac{\myW^T \tanh(\thscale \myW)}{\tanh^2(\thscale \myW)}
\end{equation}

By setting $F_x = \tanh(\thscale W_x)$, we compute the gradient of the cost with the respect to the floating point weights using the chain rule for each channel $i$:
\begin{equation}
\begin{split}
\frac{dC}{dW_i} & = \sum_{j = 0}^{C} \frac{dC}{dB_j} \frac{dB_j}{dW_i} \\
 & = \sum_{j = 0}^{C} \frac{dC}{dB_j} \frac{d(\alpha F_j)}{dW_i} \\
 & = \sum_{j = 0}^{C} \frac{dC}{dB_j} \left[\frac{d\alpha}{dW_i}F_j + \alpha\frac{d(F_j)}{dW_i}\right] \\
 & = \frac{d\alpha}{dW_i}\sum_{j = 0}^{C}\left[\frac{dC}{dB_j}F_j\right] + \alpha\frac{dC}{dB_i} \frac{d(F_i)}{dW_i}
\end{split}
\end{equation}

The computation of $\frac{d\alpha}{dW_i}$ is straightforward from Eq.~\ref{eq:alpha-tanh}.

Lastly, in the case of XNORNet, the binary weight matrix is multiplied by $\alpha$, and the convolution operation on input X is carried as:
\begin{equation}
\begin{split}
I & = (\alpha \mathrm{\textbf{B}} \circledast X) \\
  & = \alpha (\mathrm{\textbf{B}} \circledast X)
\end{split}
\end{equation}
The following CBN layer computes:
\begin{equation}
\begin{split}
\text{XNOR}(I > T, \gamma > 0) & \equiv \text{XNOR}(\alpha(\mathrm{\textbf{B}} \circledast X) > T, \gamma > 0) \\
        & \equiv \text{XNOR}((\mathrm{\textbf{B}} \circledast X) > \frac{T}{\alpha}, \gamma > 0)
\end{split}
\end{equation}

So, we can adjust CBN to take into account the scaling parameter $\alpha$ by setting $T$ to:
\begin{equation}
T^{\prime} = \frac{T}{\alpha}
\end{equation}

% \begin{figure}[ht]
% 	\centering	
% 	\includegraphics[width=\linewidth]{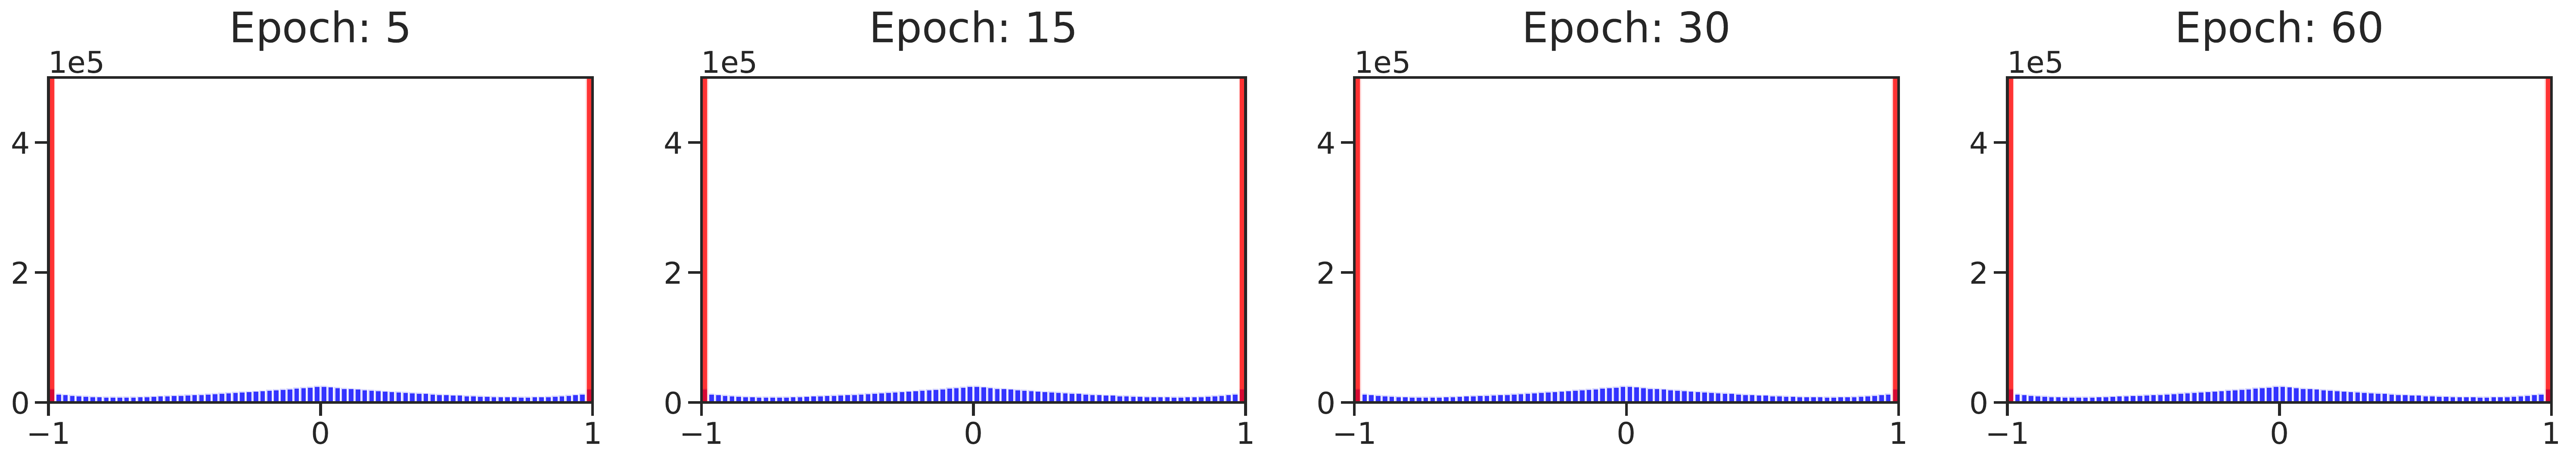}
% 	\medskip
% 	\includegraphics[width=\linewidth]{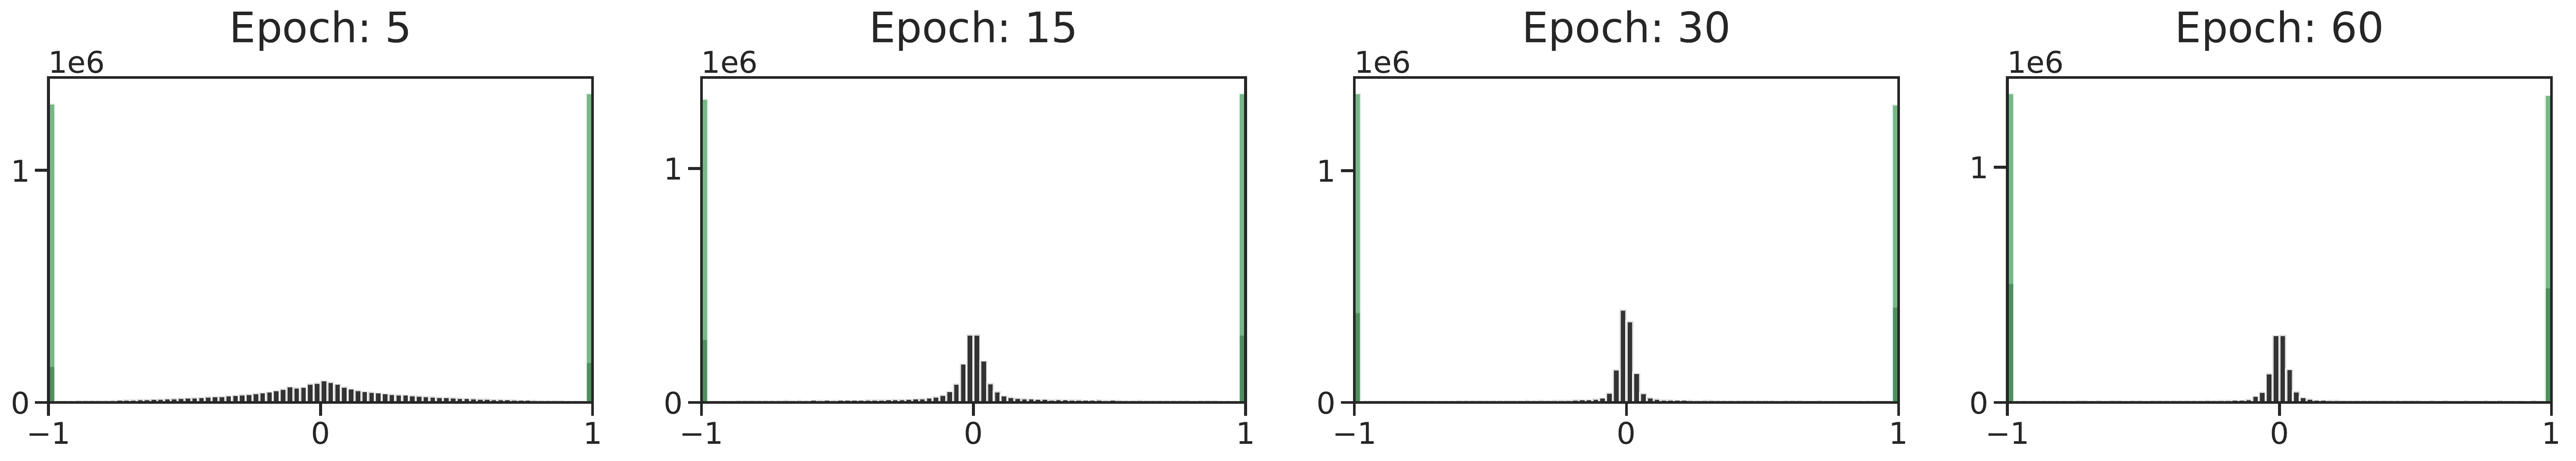}
% 	\centerline{{\small (a) Distribution of weights (top) and activations (bottom) during training for existing $\sign$-based methods.}}
% 	% FROM SIGN TRAINING
% 	\includegraphics[width=\linewidth]{Images/tanhingweights.pdf}
% 	\medskip
% 	\includegraphics[width=\linewidth]{Images/tanhingacts.pdf}
% 	\centerline{{\small(b) Distribution of weights (top) and activations (bottom) during training for our $\tanh$-based method.}}
% 	\medskip
% 	% FROM TANH TRAINING
% 	\caption{\label{fig:tanhing} \emph{Distribution of weights and activations using existing methods versus our self-binarization technique. Each plot shows two histograms, one before binarization and the other after binarization.}}
% \end{figure}

\begin{figure}[ht]
	\centering
	\begin{tabular}{c}
	\includegraphics[width=\linewidth]{Images/signweights.pdf}\\
	\includegraphics[width=\linewidth]{Images/signacts.pdf}\\
	{\small (a) Distribution of weights (top) and activations (bottom) during training for existing $\sign$-based methods.}\\
	\\
	% FROM SIGN TRAINING
	\includegraphics[width=\linewidth]{Images/tanhingweights.pdf}\\
	\includegraphics[width=\linewidth]{Images/tanhingacts.pdf}\\
	{\small(b) Distribution of weights (top) and activations (bottom) during training for our $\tanh$-based method.}
	\end{tabular}
	% FROM TANH TRAINING
	\caption{\label{fig:tanhing} \emph{Distribution of weights and activations using existing methods versus our self-binarization technique. Each plot shows two histograms, one before binarization and the other after binarization.}}
\end{figure}
